# Supplementary material for: Photoswitchable radicals as reporter spins for quantum sensing with spin defects in diamond
Source: arXiv:2510.05406 ancillary file (2025-10-06)
Supplement: Supplementary file 1 [file supporting_information.pdf]

# Supporting Information
# Photoswitchable radicals as reporter spins for quantum sensing with spin defects in diamond

Lakshmy Priya Ajayakumar[1,2], David J. Durden[1,2], Aksshay Nandakumar Regeni[1,2], Mingcai Xie[1,2], Swastik Hegde[2,3], Gustavo Aldas[1,2], Kyle Haggard[1,2], and Mikael P. Backlund[1,2,3*]

[1]*Department of Chemistry, University of Illinois at Urbana-Champaign, Urbana, Illinois 61801, USA*

[2]*Illinois Quantum Information Science and Technology Center, University of Illinois at Urbana-Champaign, Urbana, Illinois 61801, USA and*

[3]*Center for Biophysics, University of Illinois at Urbana-Champaign, Urbana, Illinois, USA**

* mikaelb@illinois.edu

## CONTENTS

A. Theory and simulation 3
   1. Sensing non-interacting quantum spins 3
   2. Classical magnetization governed by Bloch equations 9
      a. General case 9
      b. Special case: no relaxation 15
   3. Simulation of finite, fully-connected qubit network 15

B. Additional experimental details 17
   1. Covalent functionalization of diamond surface 17
   2. DEER measurements of dyes in thin polymer film 18

References 20

## A. THEORY AND SIMULATION

### 1. Sensing non-interacting quantum spins

Since in our DEER experiments the $\tau$ is fixed to be relatively short in order to isolate contributions stronger than those due to dark spins, the finite duration of the target drive $T_s$ cannot be neglected. The resulting curves are more complicated than would result from instantaneous target driving. Nevertheless, we can proceed analytically in some limiting cases. For simplicity, we do take the NV pulses to be instantaneous– a $\pi$ pulse is administered to the NV at $t = \tau$ and a final $\pi/2$ pulse is applied at $t = 2\tau$.

Figure S1 shows the basic DEER sequence employed in this work broken into four "Regions", during which the Hamiltonian is piecewise constant. Region I corresponds to $t \in (0, T_s)$, Region II to $t \in (T_s, \tau)$, Region III to $t \in (\tau, \tau + T_s)$, and Region IV to $t \in (\tau + T_s, 2\tau)$. In the first case we consider a single NV with spin $\mathbf{S}$ coupled to $N$ independent electronic spins with spin operators $\mathbf{s_j} = (s_{xj}, s_{yj}, s_{zj})^{\mathrm{T}}$ for $j \in \{1, ..., N\}$, i.e. we begin by neglecting couplings between the spin-1/2 targets. This assumption is questionable for the higher spin densities we infer from our experiments, but nonetheless lends a tractable starting point. Couplings between target spins are accounted for in an average sense in Section A 2 via finite relaxation times, and directly via finite numerical simulations in Section A 3.

In Regions I and III the target drive is on, which we take to have amplitude $\Omega$, phase $\phi_p$, and detuning $\Delta$. We invoke the rotating wave approximation and assume the interaction between each target and the NV takes an Ising form. In the appropriate multiply-rotating frame the Hamiltonian of Regions I and III is given by (in units of angular frequency):

$$\mathscr{H}_I = \sum_{j=1}^{N} \left( \mathbf{a} \cdot \mathbf{s_j} + A_j S_z s_{zj} \right), \tag{S1}$$

where $\mathbf{a} = (\Omega \cos \phi_p, \Omega \sin \phi_p, \Delta)^{\mathrm{T}}$ and $A_j$ is the coupling strength between the NV and the $j^{\mathrm{th}}$ target. In Regions II and IV the drive is off and the Hamiltonian is:

$$\mathscr{H}_{II} = \sum_{j=1}^{N} \left( \Delta s_{zj} + A_j S_z s_{zj} \right). \tag{S2}$$

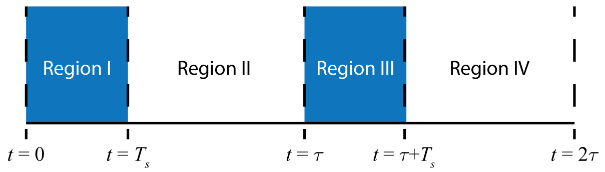


FIG. S1. Our DEER pulse sequence schematized for accompanying theoretical treatment. Target spins are driven in Regions I and II; the target drive is turned off in Regions II and IV. The NV pulses are taken to be instantaneous, with $\pi/2$ pulses occuring at $t = 0, 2\tau$ and the $\pi$ pulse at $t = \tau$.

At $t = 0$ we take the target spins to each be in the totally mixed state and the NV to be prepared in the superposition:

$$|\psi_0\rangle = \frac{1}{\sqrt{2}}\big(|0\rangle - i|{-1}\rangle\big) \tag{S3}$$

such that the initial state of the composite system is given by:

$$\rho_0 = |\psi_0\rangle\langle\psi_0| \bigotimes_{j=1}^{N} \left(\frac{\mathbb{I}_j}{2}\right), \tag{S4}$$

where $\mathbb{I}_j$ is the identity operator for the $j^{\text{th}}$ target spin. Taking advantage of the fact that the NV populations will remain unchanged until the final $\pi/2$ pulse, we decompose the system density operator at time $t$ as:

$$\rho(t) = \frac{1}{2^{N+1}}\Big(|0\rangle\langle 0| + |{-1}\rangle\langle{-1}|\Big) \bigotimes_{j=1}^{N} \mathbb{I}_j + \hat{\Upsilon}(t) + \hat{\Upsilon}^{\dagger}(t), \tag{S5}$$

such that

$$\hat{\Upsilon}(0) = \frac{i}{2^{N+1}}|0\rangle\langle{-1}| \bigotimes_{j=1}^{N} \mathbb{I}_j. \tag{S6}$$

Thus $\rho(t)$ for $t \in (0, 2\tau)$ can be obtained by propagating $\hat{\Upsilon}(t)$ through each Region. At the conclusion of Region I we have:

$$\hat{\Upsilon}(T_s) = \frac{i}{2^{N+1}}|0\rangle\langle{-1}| \bigotimes_{j=1}^{N} e^{-iT_s A_j s_{zj}}. \tag{S7}$$

At the end of Region II, just before the NV $\pi$ pulse, we have:

$$\hat{\Upsilon}(\tau) = \frac{i}{2^{N+1}} |0\rangle\langle -1| \bigotimes_{j=1}^{N} e^{-i\tau A_j s_{zj}}. \tag{S8}$$

The NV $\pi$ pulse then flips the sign of the NV coherence such that $\hat{\Upsilon}(\tau) \to -\hat{\Upsilon}(\tau)$. At $t = \tau + T_s$ we have:

$$\hat{\Upsilon}(\tau + T_s) = -\frac{i}{2^{N+1}} |0\rangle\langle -1| \bigotimes_{j=1}^{N} \left[ e^{-iT_s \mathbf{a}'_\mathbf{j} \cdot \mathbf{s}_\mathbf{j}} e^{-i\tau A_j s_{zj}} e^{iT_s \mathbf{a} \cdot \mathbf{s}_\mathbf{j}} \right], \tag{S9}$$

where we've defined $\mathbf{a}'_\mathbf{j} = \mathbf{a} - (0, 0, A_j)^\mathrm{T}$. Finally, just before the concluding NV $\pi/2$ pulse we have:

$$\hat{\Upsilon}(2\tau) = -\frac{i}{2^{N+1}} |0\rangle\langle -1| \bigotimes_{j=1}^{N} \left[ e^{-i(\tau - T_s)(\Delta - A_j) s_{zj}} e^{-iT_s \mathbf{a}'_\mathbf{j} \cdot \mathbf{s}_\mathbf{j}} e^{-i\tau A_j s_{zj}} e^{iT_s \mathbf{a} \cdot \mathbf{s}_\mathbf{j}} e^{i(\tau - T_s)\Delta s_{zj}} \right]. \tag{S10}$$

The reduced density operator of the NV just before the last $\pi/2$ pulse is obtained by tracing over the target spins in the above equation, yielding:

$$\rho_\mathrm{red}(2\tau) = \frac{1}{2}\big(|0\rangle\langle 0| + |-1\rangle\langle -1|\big) + \Upsilon_\mathrm{red}(2\tau)|0\rangle\langle -1| + \Upsilon^*_\mathrm{red}(2\tau)|-1\rangle\langle 0|, \tag{S11}$$

where the NV coherence is

$$\Upsilon_\mathrm{red}(2\tau) = -\frac{i}{2^{N+1}} \prod_{j=1}^{N} \mathrm{Tr} \left[ e^{-i(\tau - T_s)(\Delta - A_j) s_{zj}} e^{-iT_s \mathbf{a}'_\mathbf{j} \cdot \mathbf{s}_\mathbf{j}} e^{-i\tau A_j s_{zj}} e^{iT_s \mathbf{a} \cdot \mathbf{s}_\mathbf{j}} e^{i(\tau - T_s)\Delta s_{zj}} \right]. \tag{S12}$$

We alternate the phase of the final $\pi/2$ pulse between $\pm x$ and take the normalized difference of the resulting photocounts such that the end result is a signal given by:

$$\mathscr{S} = -2\mathrm{Im}\Upsilon_\mathrm{red}(2\tau). \tag{S13}$$

A small simplification to Eq. S12 can be made via the cyclic property of the trace:

$$\Upsilon_{\text{red}}(2\tau) = -\frac{i}{2^{N+1}} \prod_{j=1}^{N} \text{Tr}\left[e^{i(\tau-T_s)A_j s_{zj}} e^{-iT_s \mathbf{a}'_\mathbf{j}\cdot\mathbf{s_j}} e^{-i\tau A_j s_{zj}} e^{iT_s \mathbf{a}\cdot\mathbf{s_j}}\right]. \tag{S14}$$

We rewrite the spin of the $j^{\text{th}}$ target in terms of Pauli operators:

$$\Upsilon_{\text{red}}(2\tau) = -\frac{i}{2^{N+1}} \prod_{j=1}^{N} \text{Tr}\left[e^{i(\tau-T_s)A_j \sigma_{zj}/2} e^{-iT_s \mathbf{a}'_\mathbf{j}\cdot\boldsymbol{\sigma}_\mathbf{j}/2} e^{-i\tau A_j \sigma_{zj}/2} e^{iT_s \mathbf{a}\cdot\boldsymbol{\sigma}_\mathbf{j}/2}\right] \tag{S15}$$

in order to take advantage of the identity

$$e^{i\mathbf{v}\cdot\boldsymbol{\sigma}_\mathbf{j}} = \mathbb{I}_j \cos v + i\frac{\mathbf{v}\cdot\boldsymbol{\sigma}_\mathbf{j}}{v}\sin v, \tag{S16}$$

where $\mathbf{v} \in \mathbb{R}^3$ and $\|\mathbf{v}\| = v$. For notational convenience we introduce $\mathscr{O}_{1j}, \mathscr{O}_{2j}, \mathscr{O}_{3j}, \mathscr{O}_{4j}$ such that:

$$\Upsilon_{\text{red}}(2\tau) = -\frac{i}{2^{N+1}} \prod_{j=1}^{N} \text{Tr}\left[\mathscr{O}_{1j}\mathscr{O}_{2j}\mathscr{O}_{3j}\mathscr{O}_{4j}\right], \tag{S17}$$

$$\mathscr{O}_{1j} = e^{i(\tau-T_s)A_j\sigma_{zj}/2} = \mathbb{I}_j \cos\left(\frac{A_j(\tau-T_s)}{2}\right) + i\sigma_{zj}\sin\left(\frac{A_j(\tau-T_s)}{2}\right), \tag{S18}$$

$$\mathscr{O}_{2j} = e^{-iT_s\mathbf{a}'_\mathbf{j}\cdot\boldsymbol{\sigma}_\mathbf{j}/2} = \mathbb{I}_j\cos\left(\frac{a'_jT_s}{2}\right) - i\left(\frac{\mathbf{a}'_\mathbf{j}\cdot\boldsymbol{\sigma}_\mathbf{j}}{a'_j}\right)\sin\left(\frac{a'_jT_s}{2}\right), \tag{S19}$$

$$\mathscr{O}_{3j} = e^{-i\tau A_j\sigma_{zj}/2} = \mathbb{I}_j\cos\left(\frac{A_j\tau}{2}\right) - i\sigma_{zj}\sin\left(\frac{A_j\tau}{2}\right), \tag{S20}$$

and

$$\mathscr{O}_{4j} = e^{iT_s\mathbf{a}\cdot\boldsymbol{\sigma}_\mathbf{j}/2} = \mathbb{I}_j\cos\left(\frac{aT_s}{2}\right) + i\left(\frac{\mathbf{a}\cdot\boldsymbol{\sigma}_\mathbf{j}}{a}\right)\sin\left(\frac{aT_s}{2}\right), \tag{S21}$$

where $a = \|\mathbf{a}\| = \sqrt{\Omega^2+\Delta^2}$ and $a'_j = \|\mathbf{a}'_\mathbf{j}\| = \sqrt{\Omega^2+(\Delta-A_j)^2}$. Some algebra gives:

$$\begin{aligned}\text{Tr}\left[\mathscr{O}_{1j}\mathscr{O}_{2j}\mathscr{O}_{3j}\mathscr{O}_{4j}\right] = \quad & 2\frac{\Omega^2}{aa'_j}\cos\left(\frac{A_j(2\tau-T_s)}{2}\right)\mathcal{S}_{2j}\mathcal{S}_4 \\ & +2\cos\left(\frac{A_jT_s}{2}\right)\left[\mathcal{C}_{2j}\mathcal{C}_4 + \mathcal{S}_{2j}\mathcal{S}_4\frac{\Delta(\Delta-A_j)}{aa'_j}\right] \\ & +2\sin\left(\frac{A_jT_s}{2}\right)\left[\mathcal{C}_{2j}\mathcal{S}_4\frac{\Delta}{a} - \mathcal{S}_{2j}\mathcal{C}_4\frac{(\Delta-A_j)}{a'_j}\right],\end{aligned} \tag{S22}$$

where $\mathcal{C}_{2j} = \cos\left(a'_j T_s/2\right)$, $\mathcal{S}_{2j} = \sin\left(a'_j T_s/2\right)$, $\mathcal{C}_4 = \cos\left(aT_s/2\right)$, and $\mathcal{S}_4 = \sin\left(aT_s/2\right)$. Note that Eq. S22 does not depend on $\phi_p$. Combining Eqs. S22, S17, and S13 yields a calculable expression for the signal. Some simplifying assumptions lend further insight. If $A_j \ll a$ (weak coupling or strong driving) then $a'_j \approx a$ and Eq. S22 simplifies to:

$$\begin{aligned}\mathrm{Tr}\left[\mathscr{O}_{1j}\mathscr{O}_{2j}\mathscr{O}_{3j}\mathscr{O}_{4j}\right] \approx\ & 2\frac{\Omega^2}{a^2}\sin^2\left(\frac{aT_s}{2}\right)\cos\left(\frac{A_j\left(2\tau - T_s\right)}{2}\right) \\ & +2\left[\cos^2\left(\frac{aT_s}{2}\right) + \sin^2\left(\frac{aT_s}{2}\right)\frac{\Delta\left(\Delta - A_j\right)}{a^2}\right]\cos\left(\frac{A_jT_s}{2}\right) \\ & +2\sin\left(\frac{aT_s}{2}\right)\cos\left(\frac{aT_s}{2}\right)\left(\frac{\Delta - A_j}{a}\right)\sin\left(\frac{A_jT_s}{2}\right).\end{aligned} \tag{S23}$$

Furthermore, if $\Delta = 0$ then $a = \Omega$ and

$$\begin{aligned}\mathrm{Tr}\left[\mathscr{O}_{1j}\mathscr{O}_{2j}\mathscr{O}_{3j}\mathscr{O}_{4j}\right] \approx\ & 2\sin^2\left(\frac{\Omega T_s}{2}\right)\cos\left(\frac{A_j\left(2\tau - T_s\right)}{2}\right) \\ & +2\cos^2\left(\frac{\Omega T_s}{2}\right)\cos\left(\frac{A_jT_s}{2}\right) \\ & -2\frac{A_j}{\Omega}\sin\left(\frac{\Omega T_s}{2}\right)\cos\left(\frac{\Omega T_s}{2}\right)\sin\left(\frac{A_jT_s}{2}\right).\end{aligned} \tag{S24}$$

Application of trigonometric identities and some rearranging gives:

$$\begin{aligned}\mathrm{Tr}\left[\mathscr{O}_{1j}\mathscr{O}_{2j}\mathscr{O}_{3j}\mathscr{O}_{4j}\right] \approx\ & 2\cos\left(\frac{A_j\tau}{2}\right)\cos\left(\frac{A_j\left(\tau - T_s\right)}{2}\right) \\ & +2\sin\left(\frac{A_j\tau}{2}\right)\sin\left(\frac{A_j\left(\tau - T_s\right)}{2}\right)\cos\left(\Omega T_s\right) \\ & -\frac{A_j}{\Omega}\sin\left(\frac{A_jT_s}{2}\right)\sin\left(\Omega T_s\right).\end{aligned} \tag{S25}$$

Figure S2 depicts $\mathscr{S}$ resulting from Eqs. S17 and S25 in the case that there is only one spin coupled to the NV, i.e. $N = 1$.

If the coupling between the NV and the $j^{\text{th}}$ target spin is sufficiently weak and the interaction times sufficiently small such that $|A_j\tau|$, $|A_jT_s|$, and $|A_j(\tau - T_s)|$ are small, then a Taylor expansion of the above expression gives:

$$\mathrm{Tr}\left[\mathscr{O}_{1j}\mathscr{O}_{2j}\mathscr{O}_{3j}\mathscr{O}_{4j}\right] \approx 2\Big(1 - A_j^2 f\left(T_s;\Omega,\tau\right)\Big), \tag{S26}$$

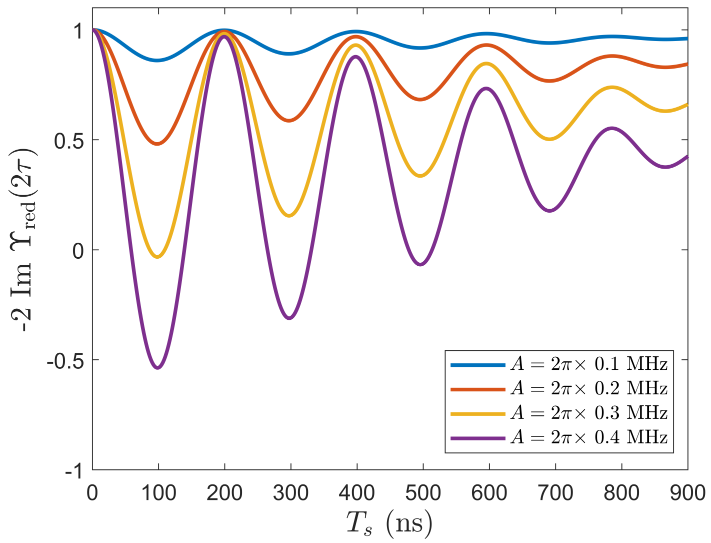


FIG. S2. Calculated signal $\mathscr{S}(T_s)$ according to Eqs. S17 and S25 in the case that the NV is coupled to only one spin, i.e. $N = 1$. Here $\tau = 900$ ns, $\Omega = \pi/(100 \text{ ns})$, and $A = A_1$.

where we've defined:

$$f\left(T_s;\Omega,\tau\right) \equiv \frac{\tau^2 + \left(\tau - T_s\right)^2}{8} - \frac{\tau\left(\tau - T_s\right)}{4}\cos\left(\Omega T_s\right) + \frac{T_s}{4\Omega}\sin\left(\Omega T_s\right). \tag{S27}$$

Referring back to Eqs. S17 and S13 then:

$$\Upsilon_{\text{red}}(2\tau) \approx -\frac{i}{2}\prod_{j=1}^{N}\left(1 - A_j^2 f\left(T_s;\Omega,\tau\right)\right) \tag{S28}$$

and

$$\mathscr{S} \approx 1 - \left(\sum_{j=1}^{N} A_j^2\right) f\left(T_s;\Omega,\tau\right), \tag{S29}$$

where again we've made use of the assumption that any one $A_j$ is small such that higher order terms can be neglected. Figure S3 depicts $\mathscr{S}(T_s)$ according to Eq. S29 for various total coupling strengths.

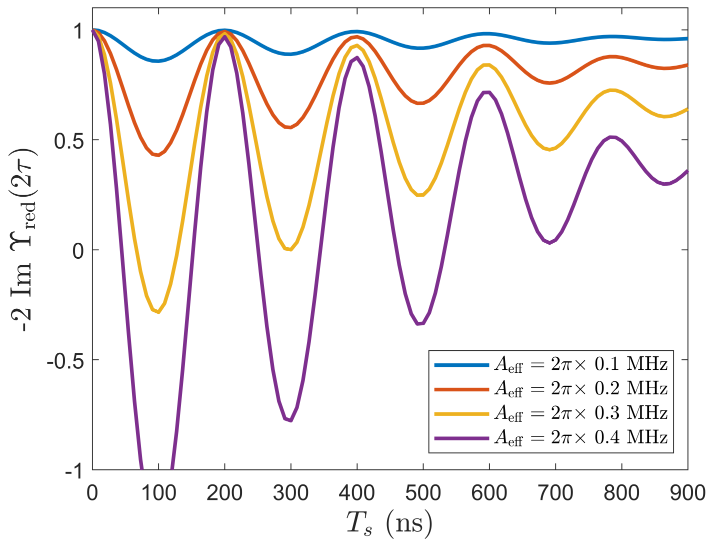


FIG. S3. Calculated signal $\mathscr{S}(T_s)$ according to Eqs. S29. Here $\tau = 900$ ns, $\Omega = \pi/(100\text{ ns})$, and $A_{\rm eff}^2 = \sum_j^N A_j^2$. The fact that $\mathscr{S} < -1$ for some $T_s$ in the strongest-coupling case is an indication that the Taylor approximation used to derive Eq. S29 is not valid in this case.

### 2. Classical magnetization governed by Bloch equations

#### *a. General case*

Here we will treat the magnetic field felt at the NV as a classical stochasic vector $\mathbf{B}(t)$ such that the time-dependent Hamiltonian in the rotating frame of the NV is given by

$$\mathscr{H}(t) = \gamma\mathbf{S}\cdot\mathbf{B}(t) \tag{S30}$$

with $\gamma$ representing the gyromagnetic ratio of the (NV) electron. We take $\mathbf{B}(t)$ to result from a classical stochastic magnetization $\mathbf{M}(\mathbf{r},t)$. Assuming again an Ising-type interaction the Hamiltonian reduces to:

$$\mathscr{H}(t) = S_z\int \mathrm{d}^3\mathbf{r}\, A(\mathbf{r})\hat{z}\cdot\mathbf{M}(\mathbf{r},t) \tag{S31}$$

where the coupling function $A(\mathbf{r})$ is given by:

$$A(\mathbf{r}) = \frac{\mu_0\gamma}{4\pi}\left(\frac{3\cos^2\theta-1}{r^3}\right). \tag{S32}$$

In each Region $\lambda \in$\{I, II, III, IV\} the NV acquires a phase

$$\Phi_\lambda = \hat{z} \cdot \int \mathrm{d}^3\mathbf{r}\, A(\mathbf{r}) \int_{t_\lambda^{(1)}}^{t_\lambda^{(2)}} \mathrm{d}t\, \mathbf{M}(\mathbf{r}, t), \tag{S33}$$

where $t_\lambda^{(1)}$ and $t_\lambda^{(2)}$ are the start and end points of Region $\lambda$, such that the total phase just before the final $\pi/2$ pulse is

$$\Phi = \Phi_{\mathrm{I}} + \Phi_{\mathrm{II}} - \Phi_{\mathrm{III}} - \Phi_{\mathrm{IV}}. \tag{S34}$$

The negative signs on the latter two phases arise due to the $\pi$ pulse administered to the NV halfway through the protocol. The final normalized difference signal is:

$$\mathscr{S} = \langle \cos \Phi \rangle \,. \tag{S35}$$

We take $\mathbf{M}(\mathbf{r}, t)$ to evolve according to the Bloch equations prescribed below. Since Eq. S31 depends only on the $z$-component of $\mathbf{M}(\mathbf{r}, t)$ we may as well proceed with our Bloch equations expressed in the rotating frame of the target magnetization. In Regions I and III the target magnetization is subject to an on-resonance drive of strength $\Omega$ and phase $\phi_p$ described by a matrix:

$$\mathbf{D} = \begin{pmatrix} 0 & 0 & \Omega \sin \phi_p \\ 0 & 0 & -\Omega \cos \phi_p \\ -\Omega \sin \phi_p & \Omega \cos \phi_p & 0 \end{pmatrix}. \tag{S36}$$

A relaxation matrix is defined:

$$\mathbf{\Gamma} = \begin{pmatrix} -1/T_2 & 0 & 0 \\ 0 & -1/T_2 & 0 \\ 0 & 0 & -1/T_1 \end{pmatrix}. \tag{S37}$$

For $\lambda \in$ \{I, II, III, IV\} the corresponding Bloch equation is

$$\dot{\mathbf{M}}(\mathbf{r}, t) = \mathbf{W}_\lambda \mathbf{M}(\mathbf{r}, t), \tag{S38}$$

where $\mathbf{W}_{\mathrm{I}} = \mathbf{W}_{\mathrm{III}} = \mathbf{D} + \mathbf{\Gamma}$, $\mathbf{W}_{\mathrm{II}} = \mathbf{W}_{\mathrm{IV}} = \mathbf{\Gamma}$ and assuming that at long times we have $\mathbf{M}(\mathbf{r}, t) \to \mathbf{0}$. We denote the stochastic initial magnetization at position $\mathbf{r}$ and time $t = t_{\mathrm{I}}^{(1)} = 0$ as $\mathbf{M_0}(\mathbf{r})$. We make the following assumptions about the first and second moments of $\mathbf{M_0}(\mathbf{r})$:

$$\langle \mathbf{M_0}(\mathbf{r}) \rangle = \mathbf{0} \in \mathbb{R}^3 \tag{S39a}$$

$$\left\langle \mathbf{M_0}(\mathbf{r}) \mathbf{M_0^{\mathrm{T}}}(\mathbf{r}') \right\rangle = \frac{\gamma^2 \hbar^2 \sigma}{4} \mathbf{I_3} \, \delta^3 \left( \mathbf{r} - \mathbf{r}' \right) \, \delta \left( u - d_{NV} \right), \tag{S39b}$$

where $\mathbf{I_3}$ is the $3 \times 3$ identity matrix, $\sigma$ is the (assumed constant) areal density of target spins on the diamond surface, and $u = \frac{1}{\sqrt{3}} z + \sqrt{\frac{2}{3}} x$ arising from the angle $\theta_t = \arctan(\sqrt{2})$ between $\hat{z}$ and the surface normal. The solution to Eq. S38 in each Region is:

$$\mathbf{M}\left(\mathbf{r}, t\right) = e^{\mathbf{W}_\lambda \left( t - t_\lambda^{(1)} \right)} \mathbf{M} \left( \mathbf{r}, t_\lambda^{(1)} \right) \tag{S40}$$

for $t \in \left( t_\lambda^{(1)}, t_\lambda^{(2)} \right)$. In Region I this gives:

$$\mathbf{M}(\mathbf{r}, t) = e^{(\mathbf{D} + \mathbf{\Gamma}) t} \, \mathbf{M_0} \left( \mathbf{r} \right), \tag{S41}$$

in Region II:

$$\mathbf{M}(\mathbf{r}, t) = e^{\mathbf{\Gamma}(t - T_s)} e^{(\mathbf{D} + \mathbf{\Gamma}) T_s} \, \mathbf{M_0}(\mathbf{r}) \tag{S42}$$

in Region III:

$$\mathbf{M}(\mathbf{r}, t) = e^{(\mathbf{D} + \mathbf{\Gamma})(t - \tau)} e^{\mathbf{\Gamma}(\tau - T_s)} e^{(\mathbf{D} + \mathbf{\Gamma}) T_s} \, \mathbf{M_0}(\mathbf{r}) \tag{S43}$$

and in Region IV:

$$\mathbf{M}(\mathbf{r}, t) = e^{\mathbf{\Gamma}(t - \tau - T_s)} e^{(\mathbf{D} + \mathbf{\Gamma}) T_s} e^{\mathbf{\Gamma}(\tau - T_s)} e^{(\mathbf{D} + \mathbf{\Gamma}) T_s} \, \mathbf{M_0}(\mathbf{r}). \tag{S44}$$

Per Eq. S33, computing the phase $\Phi_\lambda$ requires evaluating a time integral over $\mathbf{M}(\mathbf{r}, t)$. In Region I, direct integration of Eq. S41 gives:

$$\int_0^{T_s} \mathrm{d}t \, \mathbf{M}(\mathbf{r}, t) = \left( e^{(\mathbf{D} + \mathbf{\Gamma}) T_s} - \mathbf{I_3} \right) \left( \mathbf{D} + \mathbf{\Gamma} \right)^{-1} \mathbf{M_0} \left( \mathbf{r} \right). \tag{S45}$$

Similarly, integration over Region II gives:

$$\int_{T_s}^{\tau} \mathrm{d}t\, \mathbf{M}(\mathbf{r},t) = \left(e^{\boldsymbol{\Gamma}(\tau-T_s)} - \mathbf{I_3}\right) \boldsymbol{\Gamma}^{-1} e^{(\mathbf{D}+\boldsymbol{\Gamma})T_s} \mathbf{M_0}\left(\mathbf{r}\right), \tag{S46}$$

integration over Region III gives:

$$\int_{\tau}^{\tau+T_s} \mathrm{d}t\, \mathbf{M}(\mathbf{r},t) = \left(e^{(\mathbf{D}+\boldsymbol{\Gamma})T_s} - \mathbf{I_3}\right) \left(\mathbf{D}+\boldsymbol{\Gamma}\right)^{-1} e^{\boldsymbol{\Gamma}(\tau-T_s)} e^{(\mathbf{D}+\boldsymbol{\Gamma})T_s} \mathbf{M_0}\left(\mathbf{r}\right), \tag{S47}$$

and integration over Region IV gives:

$$\int_{\tau+T_s}^{2\tau} \mathrm{d}t\, \mathbf{M}(\mathbf{r},t) = \left(e^{\boldsymbol{\Gamma}(\tau-T_s)} - \mathbf{I_3}\right) \boldsymbol{\Gamma}^{-1} e^{(\mathbf{D}+\boldsymbol{\Gamma})T_s} e^{\boldsymbol{\Gamma}(\tau-T_s)} e^{(\mathbf{D}+\boldsymbol{\Gamma})T_s} \mathbf{M_0}\left(\mathbf{r}\right). \tag{S48}$$

Hence,

$$\int_{0}^{\tau} \mathrm{d}t\, \mathbf{M}(\mathbf{r},t) - \int_{\tau}^{2\tau} \mathrm{d}t\, \mathbf{M}(\mathbf{r},t) = \boldsymbol{\Xi} \cdot \mathbf{M_0}(\mathbf{r}), \tag{S49}$$

where the matrix $\boldsymbol{\Xi}$ is defined by:

$$\boldsymbol{\Xi} \equiv \left\{ \left[e^{(\mathbf{D}+\boldsymbol{\Gamma})T_s} - \mathbf{I_3}\right] \left(\mathbf{D}+\boldsymbol{\Gamma}\right)^{-1} + \left[e^{\boldsymbol{\Gamma}(\tau-T_s)} - \mathbf{I_3}\right] \boldsymbol{\Gamma}^{-1} e^{(\mathbf{D}+\boldsymbol{\Gamma})T_s} \right\} \times \left\{ \mathbf{I_3} - e^{\boldsymbol{\Gamma}(\tau-T_s)} e^{(\mathbf{D}+\boldsymbol{\Gamma})T_s} \right\}. \tag{S50}$$

Examining Eqs. S33 and S34, the total phase acquired by the NV can be re-expressed:

$$\Phi = \hat{z} \cdot \boldsymbol{\Xi} \cdot \int \mathrm{d}^3\mathbf{r}\, A(\mathbf{r}) \mathbf{M_0}(\mathbf{r}). \tag{S51}$$

Clearly $\langle \Phi \rangle = 0$. Its second moment is given by:

$$\begin{aligned} \left\langle \Phi^2 \right\rangle &= \hat{z}^{\mathrm{T}} \boldsymbol{\Xi} \left( \int \mathrm{d}^3\mathbf{r} \int \mathrm{d}^3\mathbf{r}' A\left(\mathbf{r}\right) A\left(\mathbf{r}'\right) \left\langle \mathbf{M_0}(\mathbf{r}) \mathbf{M_0^{\mathrm{T}}}(\mathbf{r}') \right\rangle \right) \boldsymbol{\Xi}^{\mathrm{T}} \hat{z} \\ &= \left(\frac{\mu_0}{4\pi}\right)^2 \frac{\gamma^4 \hbar^2 \sigma}{4} \left( \int \mathrm{d}^3\mathbf{r} \left( \frac{3\cos^2\theta - 1}{r^3} \right)^2 \delta\left(u - d_{NV}\right) \right) \left\| \boldsymbol{\Xi}^{\mathrm{T}} \hat{z} \right\|^2. \end{aligned} \tag{S52}$$

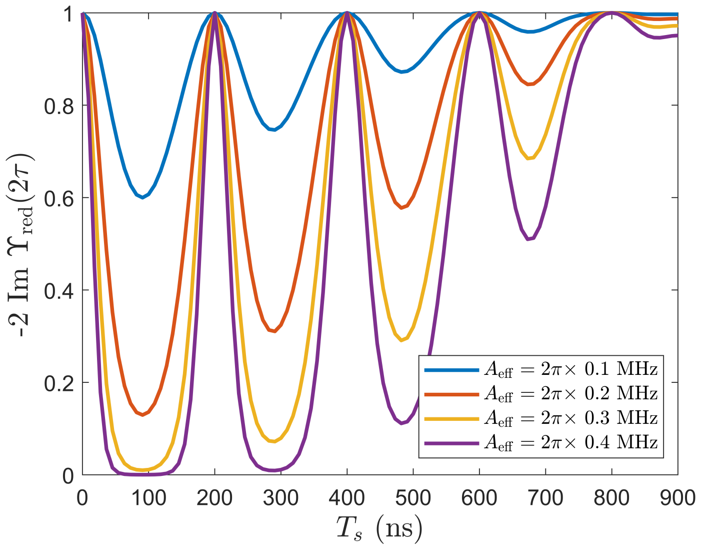


.

FIG. S4. Calculated signal $\mathscr{S}(T_s)$ according to Eqs. S54 for various $A_{\rm eff}$ and fixed $T_1 = T_2 = 100$ µs. Here $\tau = 900$ ns and $\Omega = \pi/(100\text{ ns})$

Evaluating the spatial integral above yields:

$$\langle \Phi^2 \rangle = \left(\frac{\mu_0}{4\pi}\right)^2 \frac{3\pi\gamma^4\hbar^2\sigma}{32 d_{NV}^4} \left\| \mathbf{\Xi}^{\rm T} \hat{z} \right\|^2 . \tag{S53}$$

In general, computing $\mathscr{S}$ from Eq. S35 requires higher moments of $\Phi$. If we assume that $\Phi$ is normally distributed, however, then:

$$\mathscr{S} = \langle \cos\Phi \rangle = e^{-\langle \Phi^2 \rangle/2} = \exp\left[ -\left(\frac{\mu_0}{4\pi}\right)^2 \frac{3\pi\gamma^4\hbar^2\sigma}{64 d_{NV}^4} \left\| \mathbf{\Xi}^{\rm T} \hat{z} \right\|^2 \right] . \tag{S54}$$

It's not clear that $\left\| \mathbf{\Xi}^{\rm T} \hat{z} \right\|^2$ reduces to a particularly simple form, but one can readily confirm in Mathematica that $\frac{\partial}{\partial_{\phi_p}} \left\| \mathbf{\Xi}^{\rm T} \hat{z} \right\|^2 = 0$ and thus we may as well take $\phi_p = 0$ starting with our definition of $\mathbf{D}$ in Eq. S36. Then upon specifying the other parameters of the problem, the curve $\mathscr{S}(T_s)$ can be easily computed. Figures S4, S5, and S6 show some of the variety of curve shapes consistent with Eq. S54, where we have defined an effective coupling strength $A_{\rm eff}$ such that

$$A_{\rm eff}^2 = \left(\frac{\mu_0}{4\pi}\right)^2 \frac{3\pi\gamma^4\hbar^2\sigma}{32 d_{NV}^4} . \tag{S55}$$

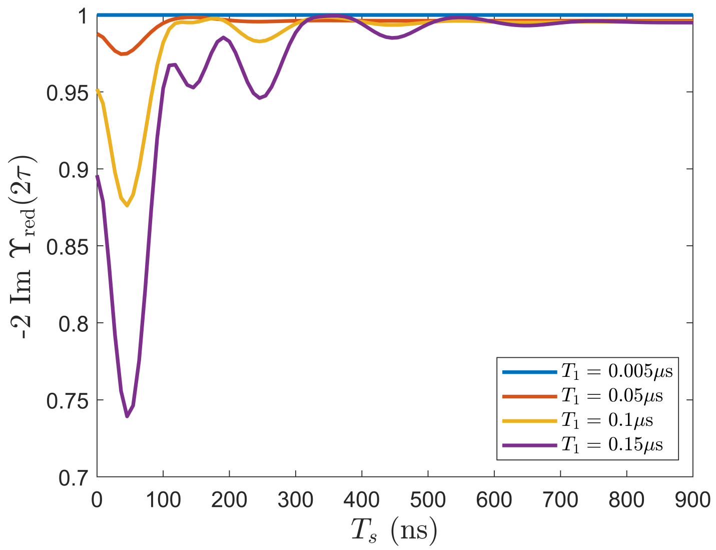


FIG. S5. Calculated signal $\mathscr{S}(T_s)$ according to Eqs. S54 for various $T_1$ and fixed $A_{\rm eff} = 2\pi \times 0.5$ MHz. The decoherence time is set to its maximum such that $T_2 = 2T_1$ in each case. Here $\tau = 900$ ns and $\Omega = \pi/(100$ ns).

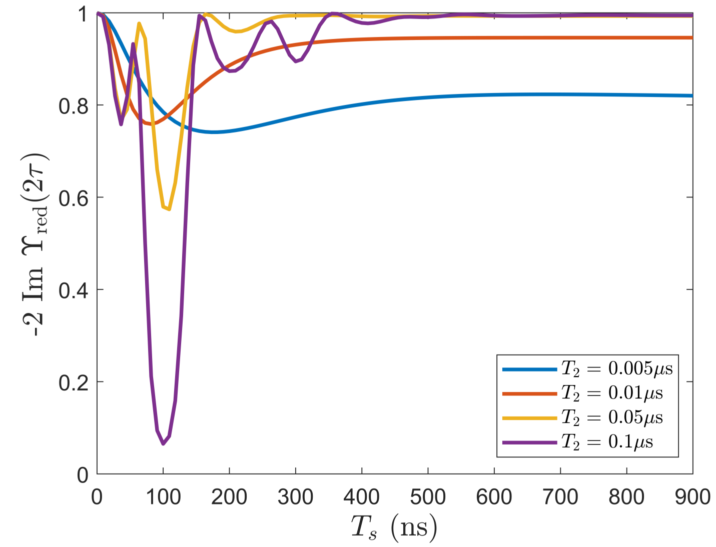


FIG. S6. Calculated signal $\mathscr{S}(T_s)$ according to Eqs. S54 for various $T_2$, fixed $A_{\rm eff} = 2\pi \times 0.5$ MHz, and fixed $T_1 = 100$ µs. Here $\tau = 900$ ns and $\Omega = \pi/(100$ ns).

### b. *Special case: no relaxation*

In the limit $T_1 \to \infty, T_2 \to \infty$ the quantity $\|\mathbf{\Xi}^{\mathrm{T}}\hat{z}\|^2$ evaluates to:

$$\left\|\mathbf{\Xi}^{\mathrm{T}}\hat{z}\right\|^2 = \frac{4}{\Omega^2}\sin^2\left(\frac{\Omega T_s}{2}\right)\left[2 + \Omega^2(\tau - T_s)^2 - 2\cos(\Omega T_s) + 2\Omega(\tau - T_s)\sin(\Omega T_s)\right]. \quad \text{(S56)}$$

For large $\Omega$ this tends to:

$$\lim_{\Omega\to\infty}\left\|\mathbf{\Xi}^{\mathrm{T}}\hat{z}\right\|^2 = 4(\tau - T_s)^2\sin^2\left(\frac{\Omega T_s}{2}\right), \quad \text{(S57)}$$

which has a maximum of approximately $4\tau^2$. Plugging this into Eq. S54 gives a signal depth of

$$\min_{T_s}\mathscr{S} \approx \exp\left[-\left(\frac{\mu_0}{4\pi}\right)^2\frac{3\pi\gamma^4\hbar^2\sigma}{16d_{NV}^4}\tau^2\right], \quad \text{(S58)}$$

which is equivalent to Eq. C15 in Ref. [1] upon noting that they define the total duration of the pulse sequence to be $\tau$ rather than $2\tau$.

## 3. Simulation of finite, fully-connected qubit network

The findings in the previous section indicate that a short target $T_2$ can explain the highly damped DEER oscillations we observed in several of our experiments. In this section we resort to numerical simulation of the quantum system to suggest a likely physical mechanism for the shortened $T_2$ values. Our simulation is carried out using a custom MATLAB program. The Hamiltonian is

$$\mathscr{H} = \Omega(t)\sum_{j=1}^{N}s_{xj} + \sum_{j=1}^{N}\mathbf{s_j}\cdot\mathbf{A_j}\cdot\mathbf{S} + \sum_{j<k}\mathbf{s_j}\cdot\mathbf{B_{jk}}\cdot\mathbf{s_k}, \quad \text{(S59)}$$

where $\Omega(t) = \Omega$ in Regions I and III and $\Omega(t) = 0$ in Regions II and IV. $\mathbf{A_j}$ is the dipolar coupling tensor connecting the NV to the $j^{\mathrm{th}}$ target spin:

$$\mathbf{A_j} = -\frac{\mu_0\gamma^2\hbar}{4\pi r_j^3}\left[\frac{3\left(\mathbf{s_j}\cdot\mathbf{r_j}\right)\left(\mathbf{S}\cdot\mathbf{r_j}\right)}{r_j^2} - \mathbf{s_j}\cdot\mathbf{S}\right], \quad \text{(S60)}$$

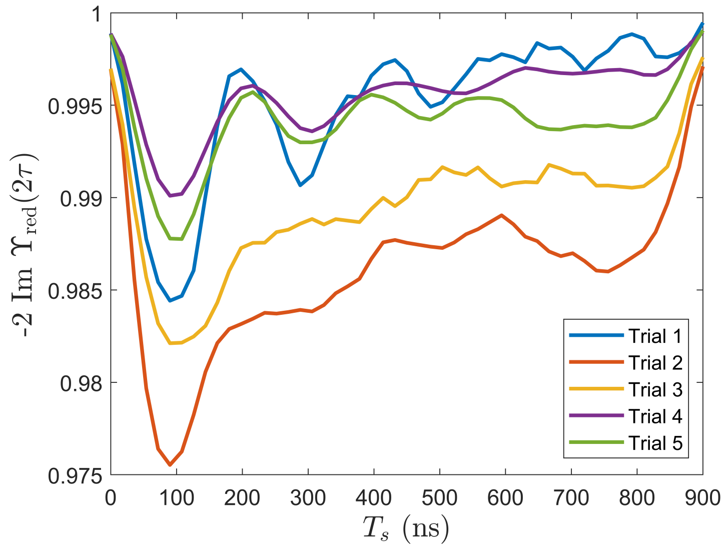


FIG. S7. Caption

with $\mathbf{r_j}$ the position vector connecting the NV and the $j^{\mathrm{th}}$ target. $\mathbf{B_{jk}}$ is the dipolar coupling tensor connecting the $j^{\mathrm{th}}$ and $k^{\mathrm{th}}$ target spins:

$$\mathbf{B_{jk}} = -\frac{\mu_0 \gamma^2 \hbar}{4\pi r_{jk}^3}\left[\frac{3\left(\mathbf{s_j}\cdot\mathbf{r_{jk}}\right)\left(\mathbf{s_k}\cdot\mathbf{r_{jk}}\right)}{r_{jk}^2} - \mathbf{s_j}\cdot\mathbf{s_k}\right], \tag{S61}$$

with $r_{jk}$ the position vector connecting the $j^{\mathrm{th}}$ and $k^{\mathrm{th}}$ targets to one another. To facilitate computation on our classical workstation we restrict the size of the system to $N = 7$. We take $d_{NV} = 12$ nm to be consistent with our average experimental NV depth. In each trial of the simulation we assign the positions of the target spins randomly throughout a square of prescribed side length. The square is positioned on the diamond surface and centered immediately above the NV. For the results depicted in Fig. S7 we took the square to have length 4 nm, corresponding to an average target density of 0.44 $\mathrm{nm}^{-2}$ on the square. We take the same initial state as in Eq. S4. Since the Hamiltonian defined in Eq. S59 is piecewise constant we can compute the propagator within each Region via direct integration before proceeding with the numerical calculation. The results of 5 independent trials are shown in Fig. S7. The key observation is that different random realizations of the target positions drawn from the same distribution can give DEER oscillations which exhibit a similar range of damping as that seen in our experiments.

Note that the shallow depth of the curves depicted in Fig. S7 is a consequence of the finite

size of the simulation: plugging the simulation parameters into Eq. S55 gives $A_{\text{eff}} \approx 2\pi \times 0.18$ MHz, which for $T_1 = T_2 = 10$ μs leads to a signal $\mathscr{S}$ with minimum around 0.25, according to Eq. S54. That even the highly damped curves from Trials 2 and 3 eventually return to near their initial points is also likely an artifact of the finite size of the simulation.

## B. ADDITIONAL EXPERIMENTAL DETAILS

### 1. Covalent functionalization of diamond surface

A concise description of this functionalization procedure is provided in the main text; here, we detail the reaction sequence. Covalent attachment of Alexa Fluor 488 dye molecules to the diamond surface was achieved using carbodiimide-mediated amide bond formation. The procedure relies on first introducing surface amine groups via activation of surface carboxylic acids, followed by coupling to the dye's N-hydroxysuccinimide (NHS) ester derivative.

Step 1: Activation of Carboxyl-Terminated Diamond Surface

Oxygen annealing of the diamond produces a heterogeneous mixture of oxygen-containing surface functional groups, including carboxylic acids (–COOH), carbonyls (C=O), and hydroxyls (–OH)[2]. Among these, the –COOH groups are the most reactive toward carbodiimide coupling and are therefore selectively targeted for chemical activation. To activate these groups for coupling, the diamond was immersed in a 2-(N-morpholino)ethanesulfonic acid (MES) buffer solution containing 100 mM 1-ethyl-3-(3-dimethylaminopropyl)carbodiimide hydrochloride (EDC) and 100 mM N-hydroxysuccinimide (NHS). EDC reacts with surface carboxylates to form an unstable O-acylisourea intermediate, which is then stabilized by NHS to generate an amine-reactive NHS ester on the diamond surface that increases the coupling efficiency and minimizes hydrolysis under aqueous conditions.

Step 2: Coupling of Ethylenediamine

After 30 minutes, the diamond was rinsed with MES buffer and immersed in a 200 mM ethylenediamine solution in the same buffer for 2 hour at room temperature. The primary amine groups of ethylenediamine nucleophilically attack the surface-bound NHS ester, forming a stable amide bond and resulting in a surface terminated with exposed amine (-$NH_2$) groups for subsequent conjugation of the dye molecules.

Step 3: Conjugation of Alexa Fluor 488

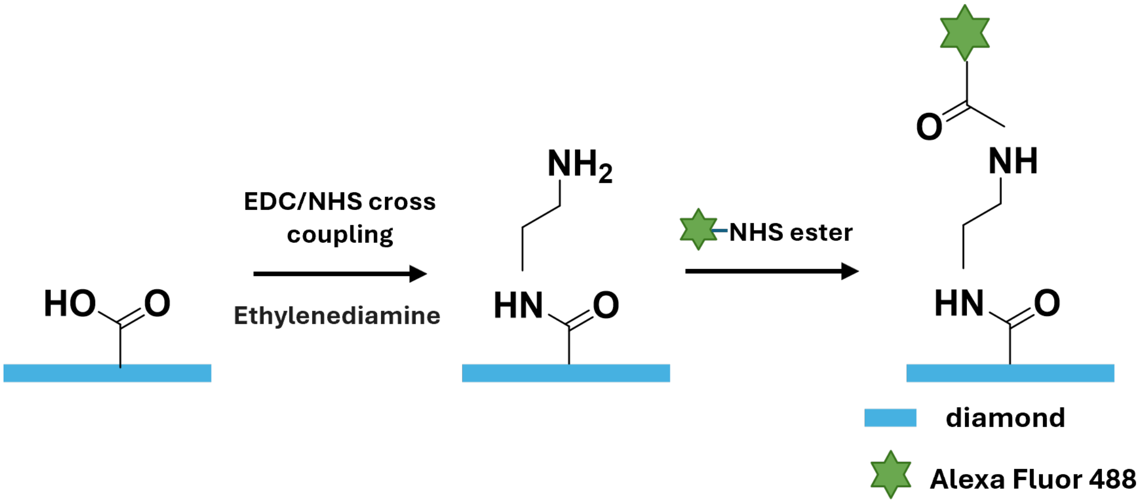


FIG. S8. Schematic of the dye functionalization reaction. Ethylenediamine was used as a linker to attach NHS-ester form of Alexa Fluor 488 molecules to the oxygen annealed diamond surface.

The amine-functionalized diamond was then rinsed with Phosphate-Buffered Saline (PBS) buffer and reacted with Alexa Fluor 488 NHS ester (50 µM, pH 7.4) for over 7 hours under gentle stirring. The NHS ester on the dye reacts selectively with surface -$NH_2$ groups, yielding a covalent amide linkage between the dye molecule and the diamond substrate. Excess dye was removed by multiple rinsing steps with PBS buffer and deionized water. FigS8 shows a schematic of the reaction steps.

### 2. DEER measurements of dyes in thin polymer film

An alternative route to surface functionalization was also employed for some DEER measurements. Alexa Fluor 488 dye was dissolved in a solution containing 1 wt % poly(methyl methacrylate) (PMMA, Sigma Aldrich 182230) in toluene to obtain a final dye concentration of 100 µM. The resulting PMMA-dye mixture was spin-coated onto the diamond substrate to form a thin film containing dispersed dye molecules. The polymer-coated diamond chip was placed in the same channel slide used for the covalently-functionalized experiments, and 50 mM MEA solution was flown in. The dye film was excited with the 488-nm laser at approximately $2 \times 10^5$ W/cm$^2$ intensity for 30 - 120 seconds to generate radicals before the DEER measurements. Figure 3E shows a DEER measurement after preparing the diamond surface in this manner. Additional examples are shown in Fig. S9. In general, we observed shallower DEER signals in measurements of polymer-coated diamond as compared to those

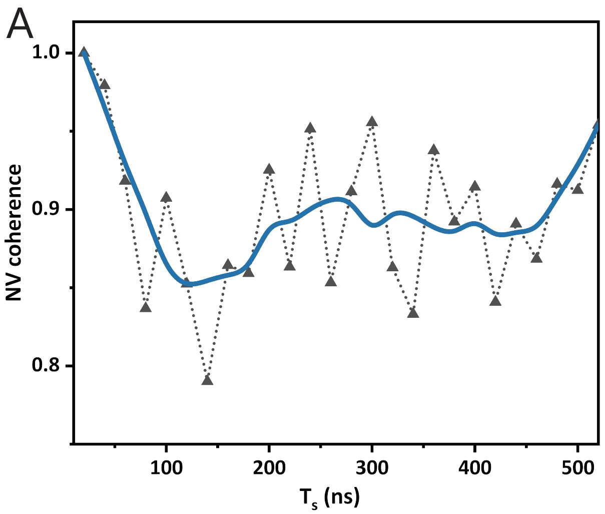


FIG. S9. DEER Rabi from dye molecules in PMMA film spin coated on the diamond surface measured with two different single NV centers.

on covalently-functionalized substrate, perhaps due to a lower obtainable surface density of radicals.

[1] B. L. Dwyer, L. V. Rodgers, E. K. Urbach, D. Bluvstein, S. Sangtawesin, H. Zhou, Y. Nassab, M. Fitzpatrick, Z. Yuan, K. De Greve, E. L. Peterson, H. Knowles, T. Sumarac, J.-P. Chou, A. Gali, V. Dobrovitski, M. D. Lukin, and N. P. De Leon, PRX Quantum **3**, 040328 (2022).

[2] S. Sangtawesin, B. L. Dwyer, S. Srinivasan, J. J. Allred, L. V. Rodgers, K. De Greve, A. Stacey, N. Dontschuk, K. M. O'Donnell, D. Hu, D. A. Evans, C. Jaye, D. A. Fischer, M. L. Markham, D. J. Twitchen, H. Park, M. D. Lukin, and N. P. De Leon, Physical Review X **9**, 031052 (2019).
